# Supplementary material for: Toward Explainable Fashion Recommendation
Source: arXiv:1901.04870 source file (2019-07-27)
Supplement: Supplementary file 1 [file supplementary.tex]

\begin{figure}[t]
\small
\centering
\begin{tabularx}{\columnwidth}{P*{2}{M}}
\toprule
\multirow{2}{*}{\begin{tabular}[]{@{}c@{}}Sample \\type\end{tabular}} & \multicolumn{2}{c}{\begin{tabular}[]{@{}c@{}}Accuracy by/\\Distribution of testing samples by\end{tabular}} \\
\cmidrule(lr){2-3}
& Score of base samples & Score gap between base and outfit flaw detection samples \\
\midrule
\begin{tabular}[]{@{}c@{}}item-\\wise\end{tabular} & \includegraphics[width=.4\columnwidth]{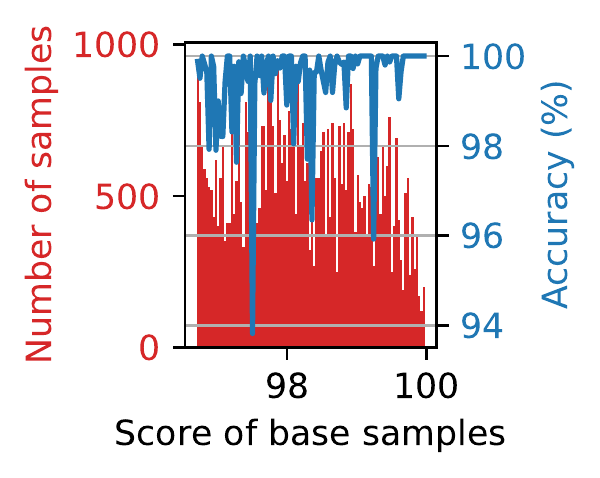} & 
\includegraphics[width=.4\columnwidth]{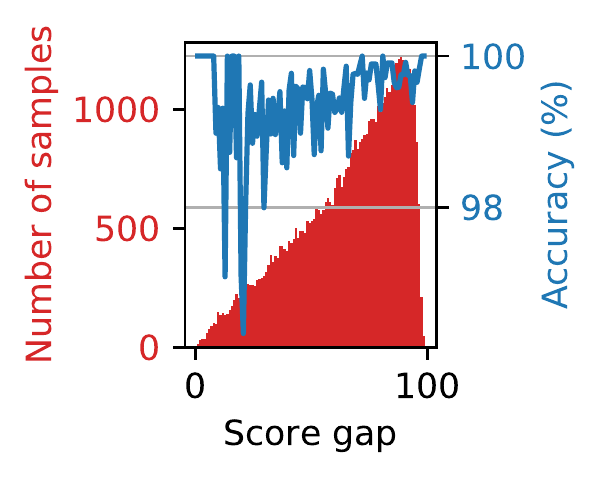} \\
\begin{tabular}[]{@{}c@{}}\textit{edge\_image}-\\wise\end{tabular} & \includegraphics[width=.4\columnwidth]{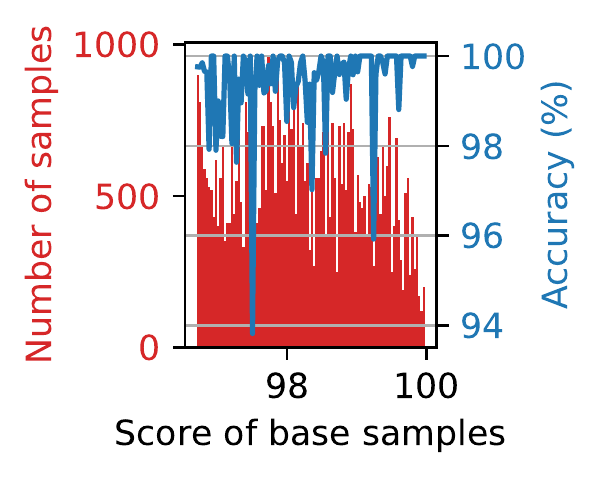} & 
\includegraphics[width=.4\columnwidth]{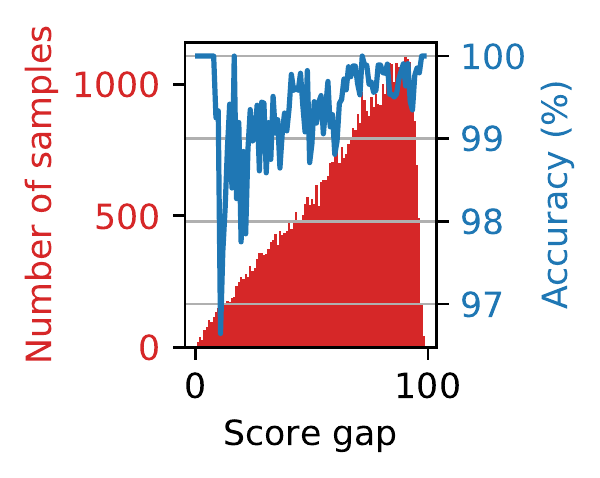} \\
\begin{tabular}[]{@{}c@{}}\textit{colors}-\\wise\end{tabular} & \includegraphics[width=.4\columnwidth]{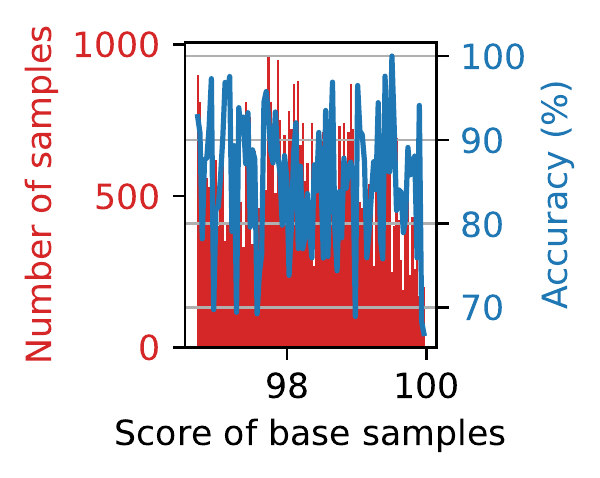} & 
\includegraphics[width=.4\columnwidth]{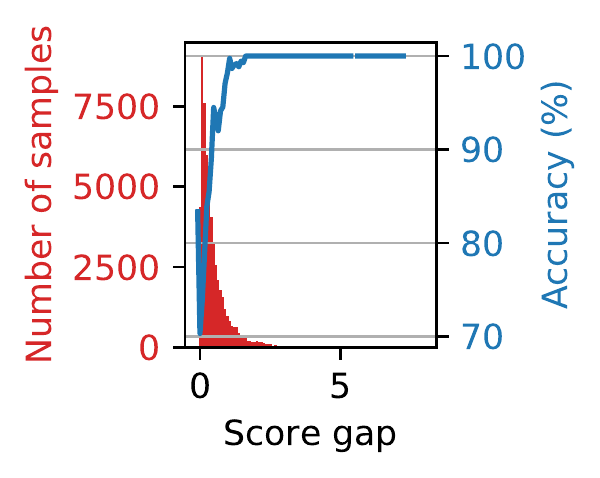} \\
\bottomrule
\end{tabularx}
\caption{Accuracy and distribution of testing samples by score of base samples and score gap between testing samples and the associated base samples. Notice the differences in value range of score gaps between \textit{colors}-wise testing samples and others.}
\label{table:accuracy_and_samples_dist_by_score_and_score_gap}
\end{figure}
